# Supplementary material for: A modular framework for collaborative human-AI, multi-modal and multi-beamline synchrotron experiments
Source: arXiv:2509.22959 source file (2025-10-02)
Supplement: Supplementary file 1 [file SI.pdf]

## *Supporting Information*

### A modular framework for collaborative human-AI, multi-modal and multi-beamline synchrotron experiments

Adam A. Corrao<sup>a</sup> (0000-0001-6111-8959), Phillip M. Maffettone<sup>a</sup> (0000-0001-7173-7972), Bruce Ravel<sup>b</sup> (0000-0002-4126-872X), Thomas A. Caswell<sup>a</sup> (0000-0003-4692-608X), Stuart I. Campbell<sup>a</sup> (0000-0001-7079-0878), Howie Joress<sup>b</sup> (0000-0002-6552-2972), Stuart I. Wilkins<sup>a</sup> (0000-0003-1191-3350), Daniel Olds<sup>a\*</sup> (0000-0002-4611-4113)

<sup>a</sup>National Synchrotron Light Source II, Brookhaven National Laboratory, Upton, NY, U.S.

<sup>b</sup>Materials Measurement Lab, National Institute of Standards and Technology, Gaithersburg, MD, U.S.

*Synchrotron, X-ray diffraction, X-ray absorption fine structure, artificial intelligence, phase mapping, combinatorial materials, multimodal*

## 60 mm diameter wafer mapping calculation

Wafer diameter = 60 mm

Beam size = 0.4 x 0.4 mm

Total measurements  $\approx$  18,000

Typical PDF measurement  $\approx$  10 seconds

**Complete map at PDF: 2 days**

Typical BMM measurement  $\approx$  10 minutes

**Complete map at BMM: 4 months**

**Figure S1.** Calculation of total measurement time needed for complete mapping of thin films sputtered on typical-sized wafers at the Pair Distribution Function (PDF) and Beamline for Materials Measurement (BMM) beamlines.

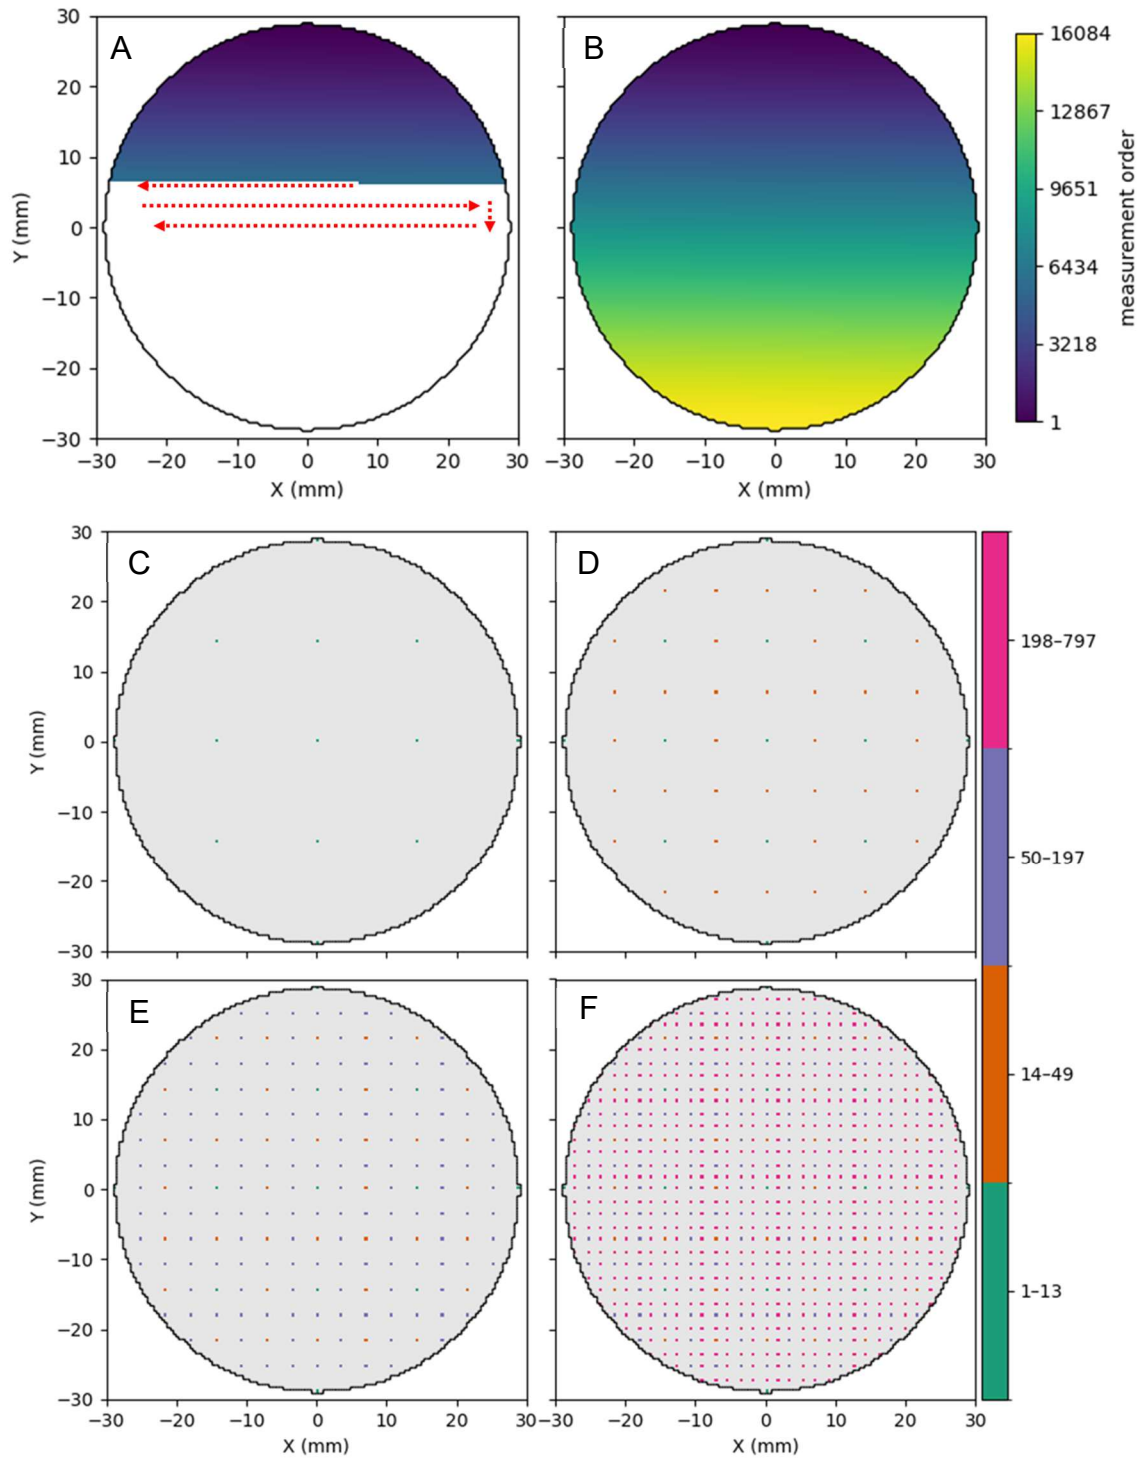

**Figure S2.** (A,B) Conventional raster scanning strategy. (A) Raster scan in progress with measurement plan shown as red arrows. (B) A complete raster scan colored by the measurement order. (C-F) A geometric series mapping strategy that demonstrates the increasing spatial resolution with subsequent series of points. Within each series of points the measurements are sampled from those that have not yet been measured.

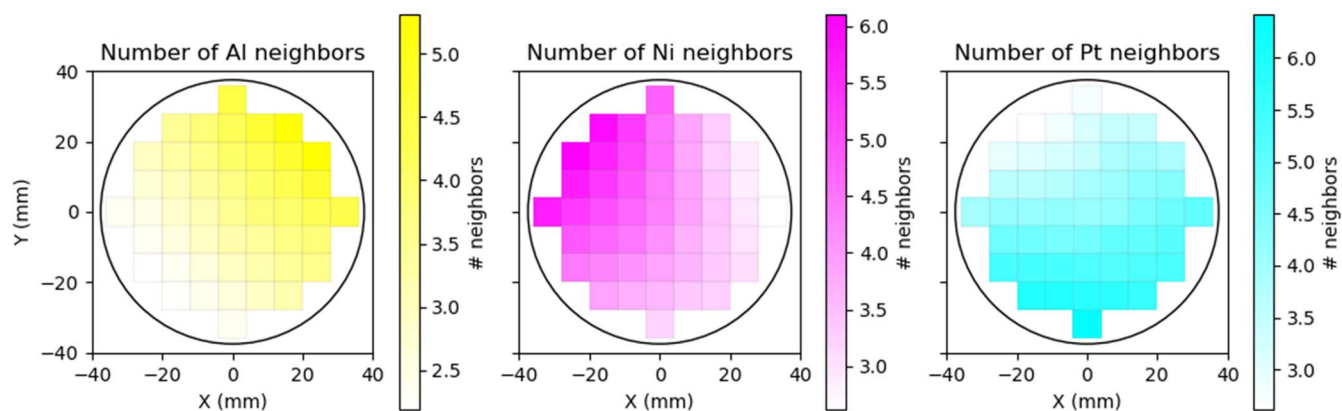

**Figure S3.** Number of Al (left), Ni (middle), and Pt (right) nearest neighbors in a face centered cubic coordination environment (12 total nearest neighbors) determined from modeling EXAFS data collected at the Pt  $L_3$  absorption edge.

### **Details of the EXAFS fitting modeling**

EXAFS analysis was performed using the Artemis program from the Demeter package.<sup>[1]</sup> A simple model was used to fit the data at each point on the wafer.

The model treats the alloy at each spot as being of the FCC structure with the first coordination shell randomly populated by the 3 metals. The coordination numbers of the Ni and Pt scatterers are parameters of the fit, while the number of Al scatterers is constrained to force the number of scatterers to equal 12. We allowed the Pt-scatterer distance,  $\delta r$ , to vary for each scatterer type. This allows the fit to accommodate local structural disorder due to the different sizes of the three atomic species. An energy shift,  $E_0$ , is applied to each scatterer. These parameters for coordination number,  $\delta r$ , and  $E_0$  account for 6 of the 7 parameters floated in the analysis.

This simple model does not properly account for the full scope of the local structural disorder about the absorber atom. The actual local structure would surely consist of some complex, non-Gaussian distribution of each of the three scatterer species. It is also likely that the details of these distributions would change with elemental concentration across the combinatorially deposited film. In the absence of a molecular dynamics simulation to assess the extent of distributional disorder, there is no practical way to model it in this analysis.

As a consequence, it was difficult to extract statistically meaningful results for  $S_0^2$  or for the  $\sigma^2$  values for each scatterer species. As a result,  $S_0^2$  was fixed to 1 and a single fitted parameter for  $\sigma^2$  was used for all three scatterer types. This surely introduces some systematic error in the determination of the three coordination numbers, which are three principal results of this analysis. Acknowledging this, we find that our model provides defensible results across the entire ensemble of EXAFS data.

For each data set, the fit was performed in R-space, the k-range of the Fourier transform was  $3 \text{ \AA}^{-1} - 11 \text{ \AA}^{-1}$ , and the fit was evaluated from  $1 \text{ \AA}$  to  $3.2 \text{ \AA}$ , a range sufficient to cover the full contribution from the first coordination shell. Each fit was evaluated using k-weighting of 1, 2, and 3, which is the default behavior in the Artemis program. The split peak seen in Figure S4A does not indicate that a scatterer lies well beyond the average first shell distance. Rather it is the result of the elevated presence of Pt scatterers

at the spot in the film, resulting in a Ramsauer-Townsend effect.<sup>[2]</sup> Figure S4B shows a spot with less Pt, resulting in a less pronounced effect. This effect on the EXAFS data is computed by FEFF<sup>[3]</sup> and incorporated into the analysis.

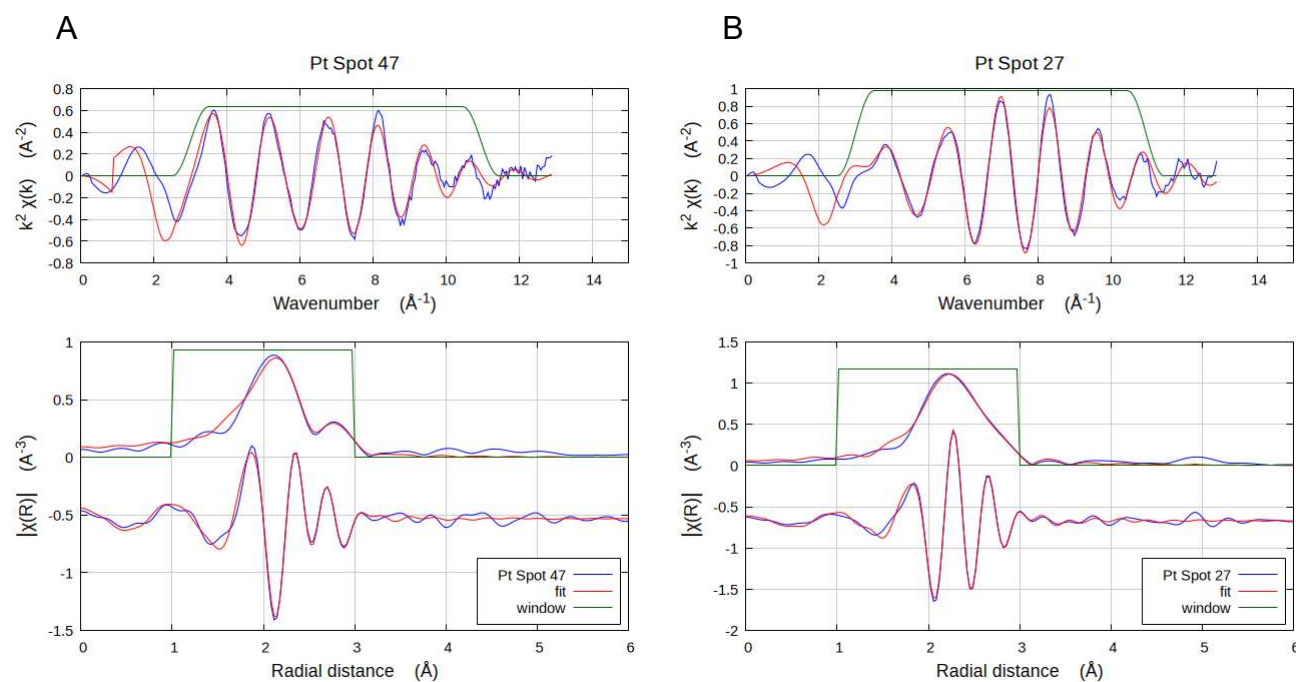

**Figure S4.** Examples of the fit quality for the Pt L<sub>3</sub>-edge EXAFS data modeled assuming 12 nearest neighbors as would be expected for face centered cubic metals. The number of Al, Ni, and Pt nearest neighbors are refined while constraining the total number of nearest neighbors to be 12. Plot A is at a Pt-rich spot, plot B is at a Pt-poor spot.

## **Complexities in Al-Ni-Pt thin film synchrotron diffraction data**

X-ray diffraction measurements on the Al-Ni-Pt thin film were done approximately 1.2 mm apart, providing a high-resolution map consisting of 1876 points. Visualizing the summed intensity from each diffraction pattern collected on the film (Figure S6) shows that intensity is highest at the top of the wafer and lowest at the bottom. This behavior may seem counterintuitive because the intensity is inversely related to the scattering power at each point (inferred from EXAFS results in Figure 6D), but the trend follows expectation from the X-ray absorption coefficients of the elements present. Given our incident beam energy of 74.46 keV ( $\lambda = 0.1665 \text{ \AA}$ ) Al and Ni transmit more than 90 % of the X-rays, while Pt absorbs approximately 50 %, thus the measured intensity should be lowest in the Pt-rich region near the bottom of the wafer as was observed.

Changes in peak positions can provide insight to alloying behavior within a crystallographic phase, such that the peaks will shift to lower  $2\theta$  angles (larger  $d$ -spacings) as the average unit cell expands and to higher  $2\theta$  angles (smaller  $d$ -spacings) as the unit cell contracts. Overlaying a subset of diffraction patterns collected along a vertical line from the bottom of the wafer to the top (Figure S5A) shows that the most intense peak at  $\approx 4.4^\circ$  ( $2\theta$ ) shifts to lower angles as the vertical position increases. This suggests that within this phase Al (1.43  $\text{\AA}$  atomic radius) substitutes for Ni (1.24  $\text{\AA}$  atomic radius) and Pt (1.385  $\text{\AA}$  atomic radius), resulting in a larger average unit cell volume. A similar shift in peak positions is observed in a horizontal line scan from the left side of the film to the right (Figure S5B), indicating similar behavior as Al replaces both Ni and Pt. However, this single peak is only a simple proxy for alloying within one phase, assumes chemical substitution on crystallographic sites, and does not account for occupancy of interstitial sites which will impact the unit cell shape and size in a less straightforward manner (*e.g.*, symmetry breaking, crystallographic direction-dependent expansion and contraction). Further, we observe many sets of peaks appearing and disappearing as a function of position on the thin film (Figure S5), indicating multiple phases are present and that a single phase, much less a single peak, cannot adequately describe this system.

Prior studies of the Al-Ni-Pt ternary system and the various binaries (*e.g.*, Ni-Pt, Al-Pt) suggest that we should observe both single-phase and multi-phase regions on the thin film, with cubic intermetallic phases ( $L1_2$  AuCu<sub>3</sub>-type,  $Pm\bar{3}m$ , space group #221) present where one element is dominant, a solid-solution tetragonal phase ( $L1_0$  AuCu-type,  $P4/mmm$ , space group #123) present when the composition is nearly equiatomic, and a mixture of these phases as well as related variants (*e.g.*, disordered *vs.* ordered, symmetry distorted) depending on the exact composition.<sup>[4–12]</sup> However, prior experimental work on these systems was done on bulk samples prepared at high temperatures ( $> 900^\circ\text{C}$ ) and typically involved post-synthesis annealing on the timescale of days to weeks to facilitate the determination of phase equilibria. In comparison, our films were prepared by sputter deposition and are expected to not be at equilibrium given the rapid cooling rates (up to  $10^9 \text{ K / s}$ ).<sup>[13,14]</sup> Further, detailed crystallographic analyses are limited, and determination of lattice parameters as a function of composition has only been done for a limited set of discrete compositions, such as the work of Meininger *et al.*<sup>[11]</sup> in which the Al content was fixed at 25 % while Ni and Pt content were varied. Given the dearth of relevant literature precedent and poorly established relationship between composition and structure (*i.e.*, existing phase diagrams are unreliable here), we used peak indexing methods, pattern matching, and trial refinements to guide our analysis.

We find that both face-centered cubic ( $Fm\bar{3}m$ , space group #225) and face-centered tetragonal ( $P4/mmm$ , space group #123) phases are present on the film (Figure S5), and that the presence of one or both phases is difficult to distinguish due to severe peak overlap and ambiguity in relative intensity contributions. The lattice parameter of the FCC phase varies from 3.70  $\text{\AA}$  to 3.82  $\text{\AA}$  (Figure S7), while the lattice parameters of the FCT phase vary from 3.75  $\text{\AA}$  to 3.93  $\text{\AA}$  and 3.4  $\text{\AA}$  to 3.76  $\text{\AA}$  for  $a$  and  $c$ , respectively. The

presence of these two phases is unexpected in relation to a review and refinement of the Al-Ni-Pt phase diagram by Grushko and Kapush<sup>[9]</sup> in which the only face-centered cubic phase reported has a lattice parameter approximately 50 % larger (5.86 Å – 5.92 Å) than we observe. We find that some of the low-angle ( $< 4^\circ 2\theta$ ) peaks can be indexed to the face-centered tetragonal ( $P4/mmm$ , space group #141) phase, but do not observe the expected  $Pm\bar{3}m$  phase or other structure types. However, peak intensities vary substantially and cannot be modeled well by structure refinement, even when March-Dollase corrections for preferred-orientation are applied or Pawley fits, in which peak intensities are freely refined, are used (Figure S7-S9). We also find that conventional isotropic peak broadening models for crystalline domain size ( $\cos\theta$  dependent) and lattice strain ( $\tan\theta$  dependent) fail to model the pattern of peak broadening well (Figure S9). A phenomenological model of anisotropic (*i.e.*,  $hkl$ -dependent) strain broadening<sup>[15]</sup> is similarly unable to fit the peak profiles well and introduces additional complexity for interpreting the results due to its lack of physicality (Figure S9).

These complicating factors led us to revisit the 2D diffraction images that are azimuthally integrated (*i.e.*, about a Debye-Scherrer cone projected onto the area detector as a ring) to conventional 1D patterns. We first show a normalized and background-subtracted image collected near the Ni deposition site that demonstrates nearly homogeneous intensity as a function of azimuthal angle (Figure S10A). This behavior is confirmed by overlaying the 1D patterns obtained from separately integrating  $90^\circ$  azimuthal slices (Figure S10B). In comparison, an image collected near the center of the sample reveals strong intensity variation as a function of azimuthal angle on select peaks at low angles (Figure S10C). Further, the variation in intensity is confirmed by the relative intensities in 1D patterns integrated from separate azimuthal slices (Figure S10D). The textured peak at  $\approx 3.5^\circ (2\theta)$  corresponds to the face-centered tetragonal phase and varies in intensity by up to approximately 50 %, suggesting phase-specific texturing.

To assess the azimuthal variation in intensity across the sample, we normalized and background-subtracted the 2D images, then used azimuthal slices from  $40^\circ - 50^\circ$  and  $130^\circ - 140^\circ$  to separately integrate patterns for comparison. Overlaying the 1D patterns obtained from integrating different azimuthal ranges (Figure S11) shows that the azimuthal variation in intensity differs depending on the measurement location as well as the  $2\theta$  range compared. For example, data collected near the Al deposition (Figure S11A) shows a minimal difference in intensity between the two azimuthal slices across nearly the full  $2\theta$  range, while data collected near the Ni deposition (Figure S11B) has the largest difference in intensity on the most intense peak at approximately  $4^\circ 2\theta$ . In comparison, data collected near the Pt deposition (Figure S11C) shows intensity varying in two distinct  $2\theta$  ranges that we define as region of interest (ROI) 1 ( $2.5^\circ - 3.9^\circ$ ) and ROI 2 ( $3.9^\circ - 6.1^\circ$ ).

To more effectively compare intensity variation across the sample, we calculated a texture coefficient for each point by dividing the summed intensity of the pattern integrated over an azimuthal range of  $130^\circ - 140^\circ$  by the summed intensity of the pattern integrated over an azimuthal range of  $40^\circ - 50^\circ$ . First, we calculated the texture coefficient over the full  $2\theta$  range (Figure S12A) and found it was at most approximately 10 %. Generally, the texture coefficient was lower than 1 on the lower left side near the Pt deposition and higher than 1 on the left side of the wafer closer to the Ni deposition site. Next, we calculated the texture coefficient comparing summed intensity in the  $2\theta$  range of ROI 1 ( $2.5^\circ - 3.9^\circ$ ) which is sensitive to the low-angle face-centered tetragonal peaks that were observed to be most highly textured in 2D images. A map of the texture coefficient from ROI 1 (Figure S12B) shows up to a nearly 50% variation in intensity, with the highest values closest to the Ni deposition site and lowest values closest to the Pt deposition site. This suggests that the phase-specific texturing hypothesized from the variation in intensity observed in 2D images is plausible and a source of considerable uncertainty in the structure, composition, and relative abundance of the corresponding phase. Lastly, we calculated the texture coefficient using ROI 2 ( $3.9^\circ - 6.1^\circ$ .) which encompasses the most intense peak that is shared by both the face-centered cubic and textured face-centered tetragonal phases (Figure S12C). This texture map shows

up to approximately a 25 % variation in intensity as a function of azimuthal angle, with the highest variation found near the center of the sample. Comparing the texture maps calculated using the full  $2\theta$  range, ROI 1, and ROI 2 (Figure S12A-C) demonstrates that significant variations in intensity as a function of azimuthal angle are present at nearly all locations on the wafer. Additionally, the specific peaks that are textured varies with position. Due to the overlap of peaks belonging to the face-centered cubic phase with those of the face-centered tetragonal phase as well as the strong texturing observed, the extraction and modeling of peak intensities to determine phase compositions and relative phase fractions is not reliable.



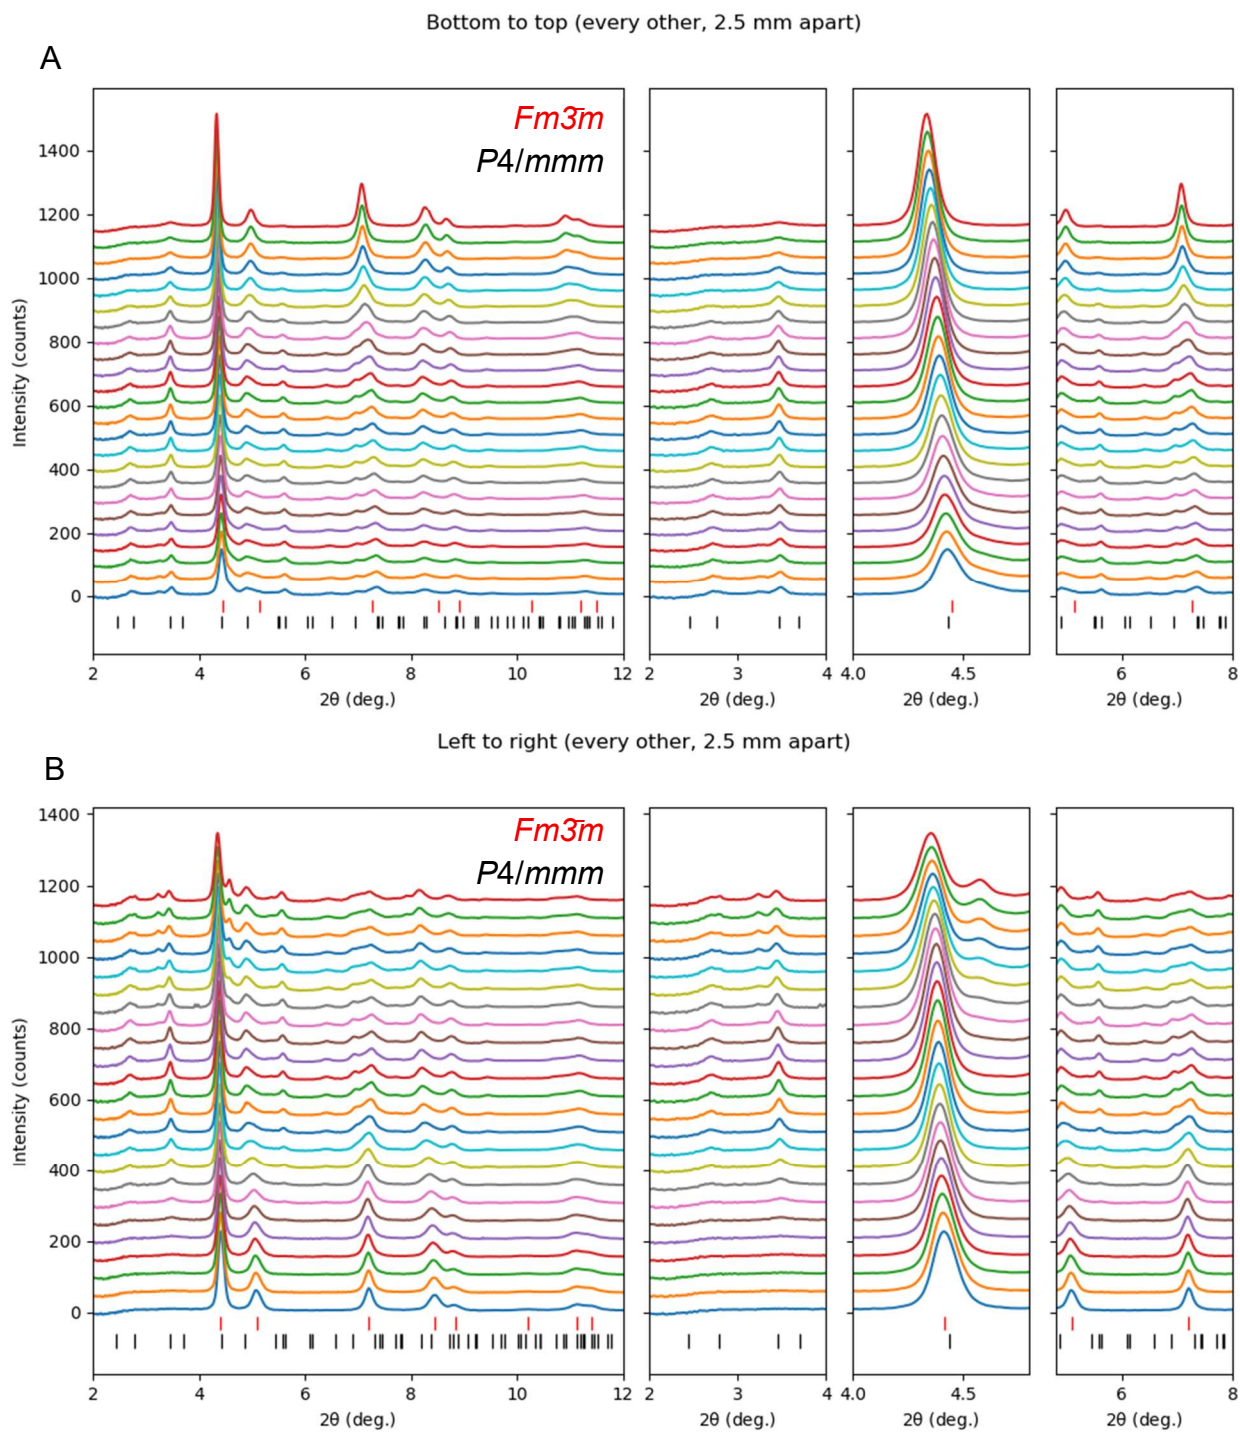

**Figure S5.** Overlay of normalized and background-subtracted diffraction patterns collected on the Al-Ni-Pt thin film ( $\lambda = 0.1665 \text{ \AA}$ ). Red and black tick marks indicate peak positions for the face-centered cubic (space group #225,  $Fm\bar{3}m$ ,  $a = 3.7795(17) \text{ \AA}$ ) and face-centered tetragonal (space group #123,  $P4/mmm$ ,  $a = 3.9048(19) \text{ \AA}$ ,  $c = 3.5319(18) \text{ \AA}$ ) phases, respectively, determined from a two-phase Rietveld fit to the pattern collected at the wafer center. Patterns are vertically offset by 50 for visualization purposes. Displayed patterns were collected approximately 2.5 mm apart. (A) Every other pattern from bottom to top on the wafer at  $x = 0.6 \text{ mm}$ . (B) Every other pattern from left to right on the wafer at  $y = 0.6 \text{ mm}$ .

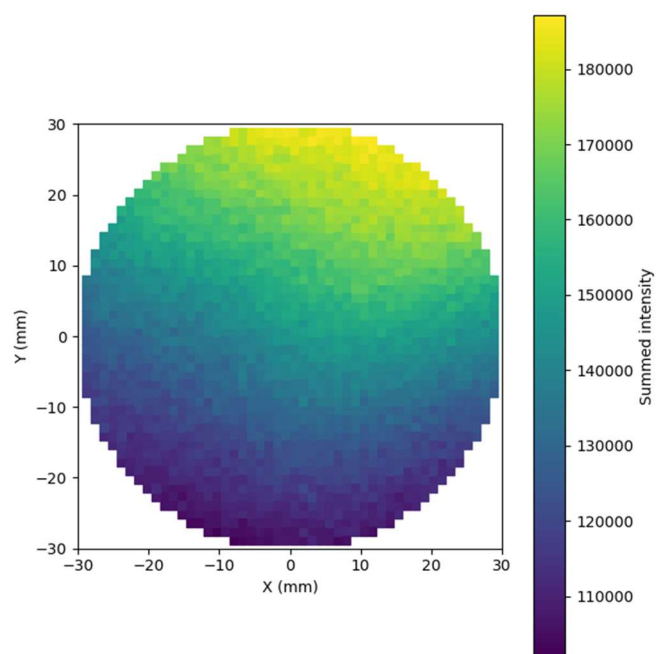

**Figure S6.** A map of summed diffraction pattern intensity showing total intensity is highest at the top of the wafer and lowest at the bottom.

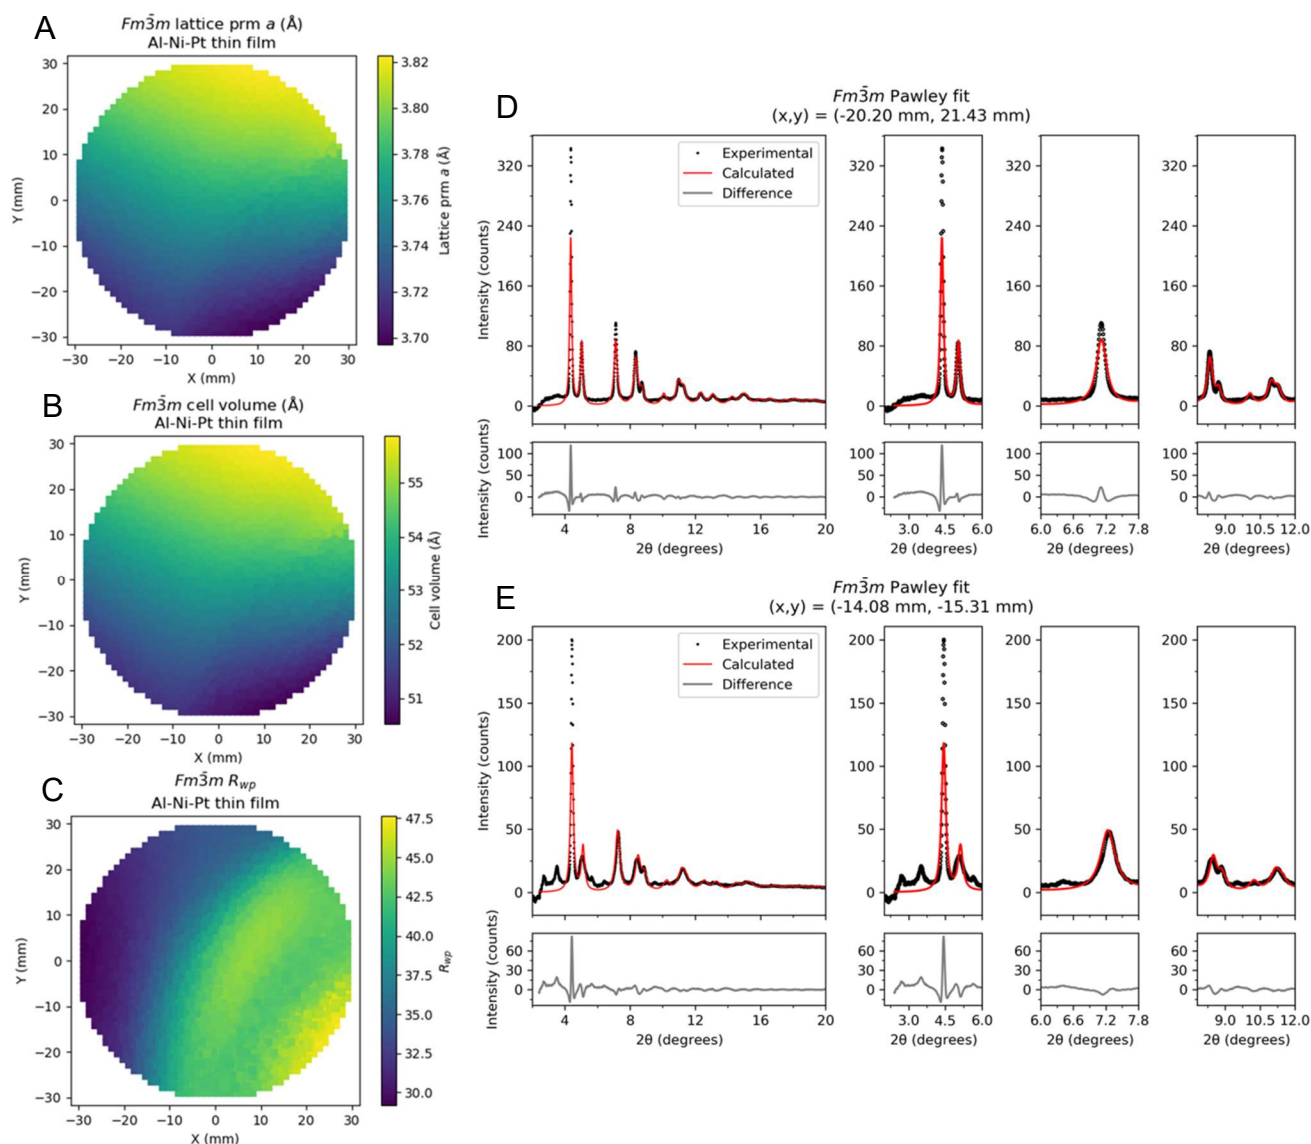

**Figure S7.** X-ray diffraction ( $\lambda = 0.1665 \text{ Å}$ ) mapping results extracted by Pawley refinement using a face-centered cubic (space group #225,  $Fm\bar{3}m$ ) solid-solution phase. (A) Unit cell lattice parameter  $a$  (Å). (B) Cell volume (Å<sup>3</sup>) (C) Weighted profile R factor ( $R_{wp}$ ). (D) Example of fit quality in upper left region with lowest  $R_{wp}$ . (E) Example of fit quality in lower left region where  $R_{wp}$  is relatively high.

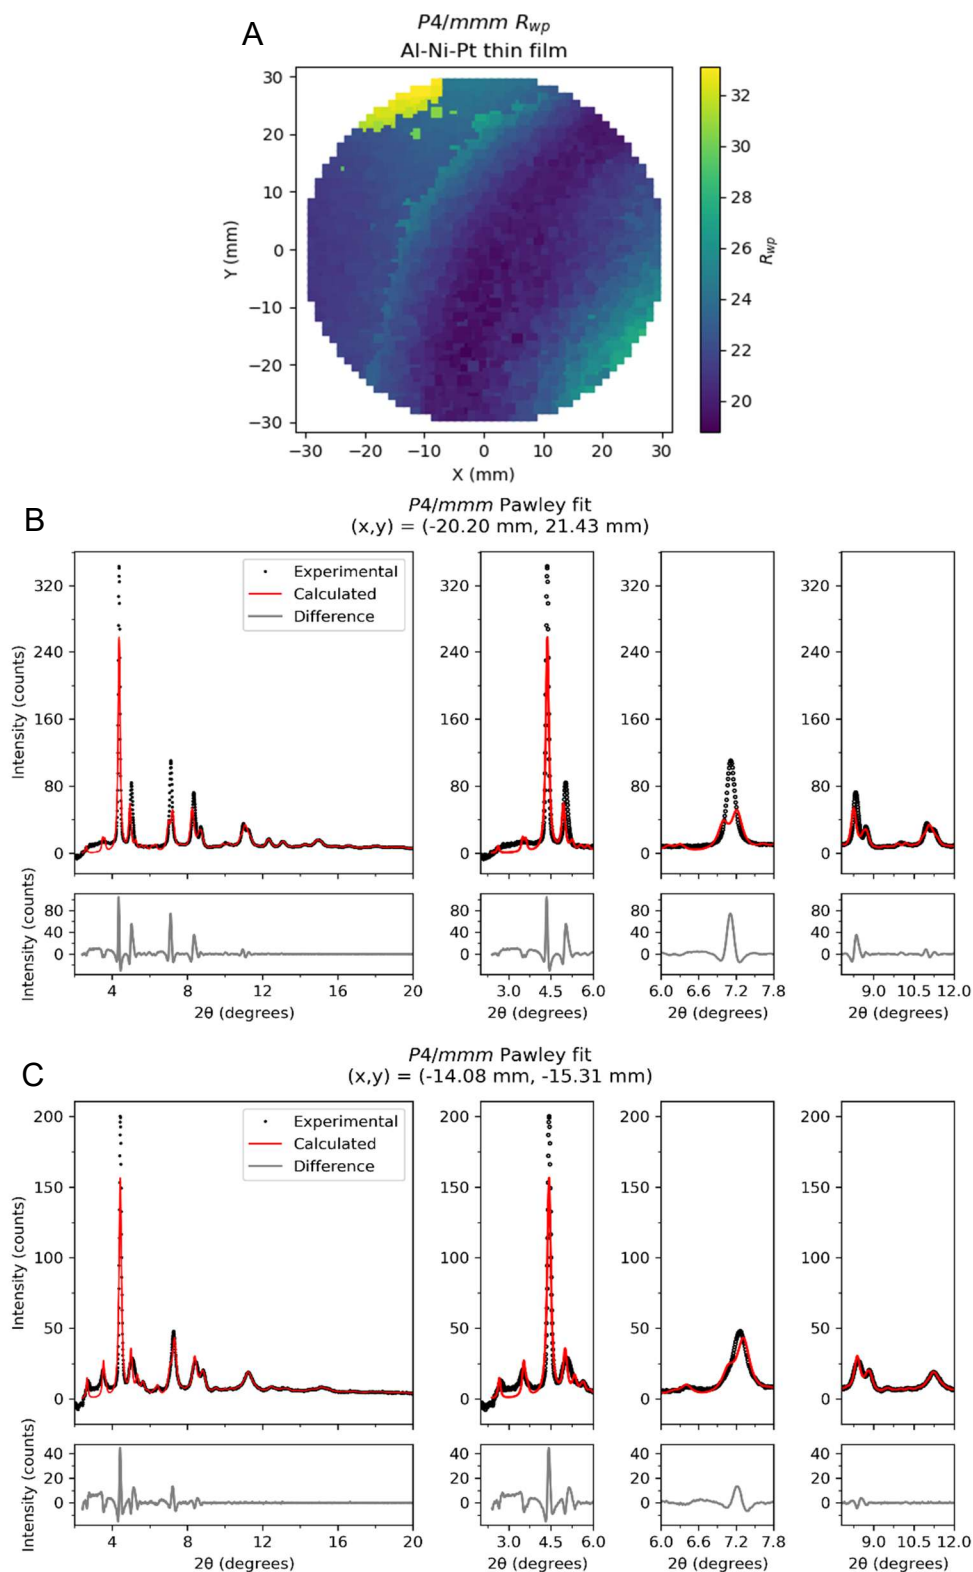

**Figure S8.** Additional X-ray diffraction ( $\lambda = 0.1665 \text{ \AA}$ ) mapping results extracted by Pawley refinement using a face-centered tetragonal (space group #123, *P4 / mmm*) solid-solution phase. (A) Weighted profile R-factor ( $R_{wp}$ ). (B) Example of fit quality in upper left region with highest  $R_{wp}$ . (C) Example of fit quality in lower left region where  $R_{wp}$  is relatively low.

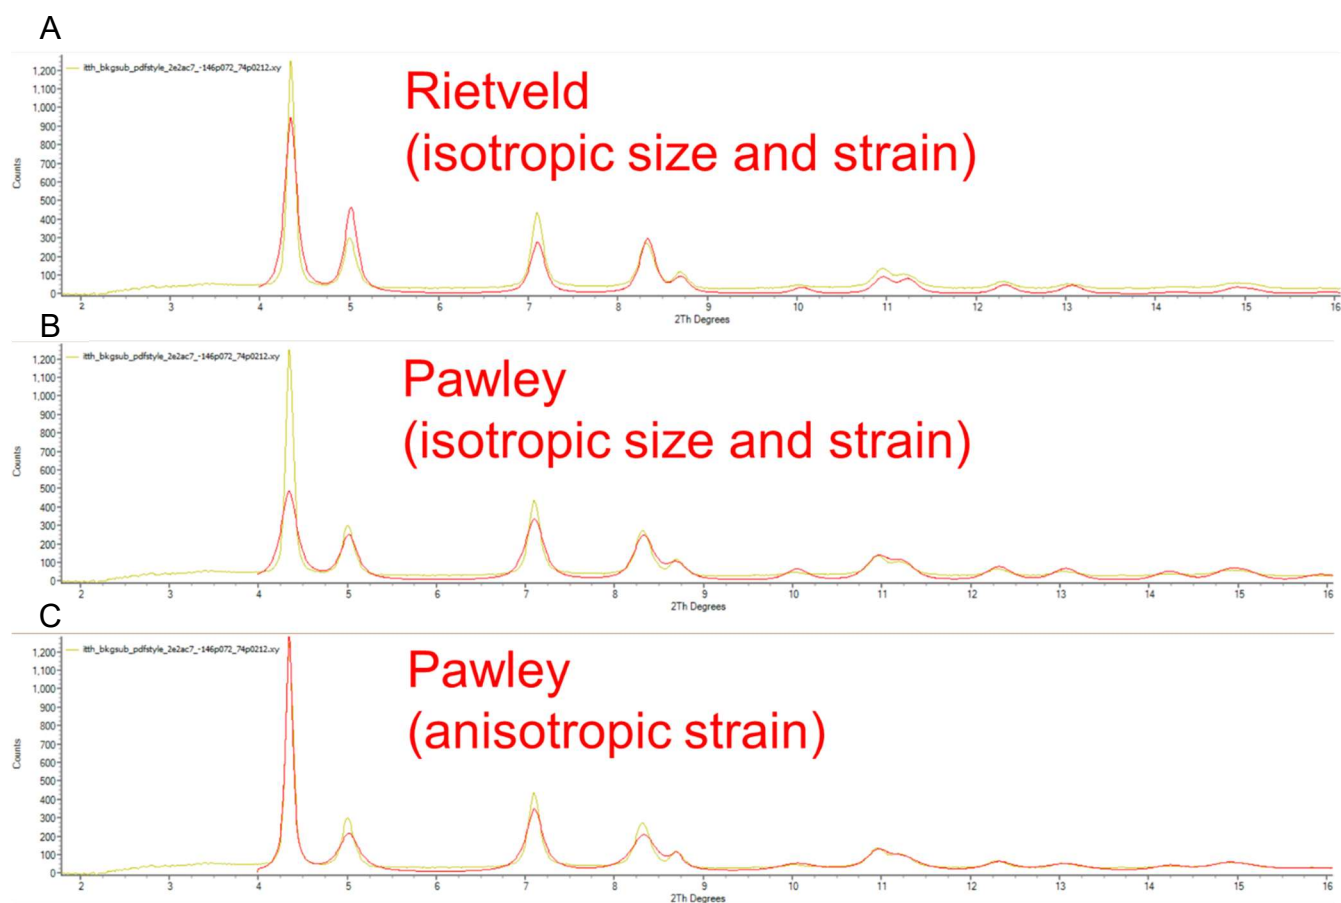

**Figure S9.** Example of issues encountered in modeling the diffraction peak intensities and peak shapes for data collected ( $\lambda = 0.1665 \text{ \AA}$ ) near the Ni deposition site on the Al-Ni-Pt combinatorial library. (A) Rietveld fit with a face-centered cubic ( $Fm\bar{3}m$ , space group #225) structural model, and isotropic size and isotropic strain terms to model peak broadening. (B) Pawley fit (freely refined intensities) with a face-centered cubic ( $Fm\bar{3}m$ , space group #225) unit cell model for peak positions, and isotropic size and isotropic strain terms to model peak broadening. (C) Pawley fit with a face-centered cubic ( $Fm\bar{3}m$ , space group #225) unit cell model for peak positions, and an anisotropic strain model for peak broadening.



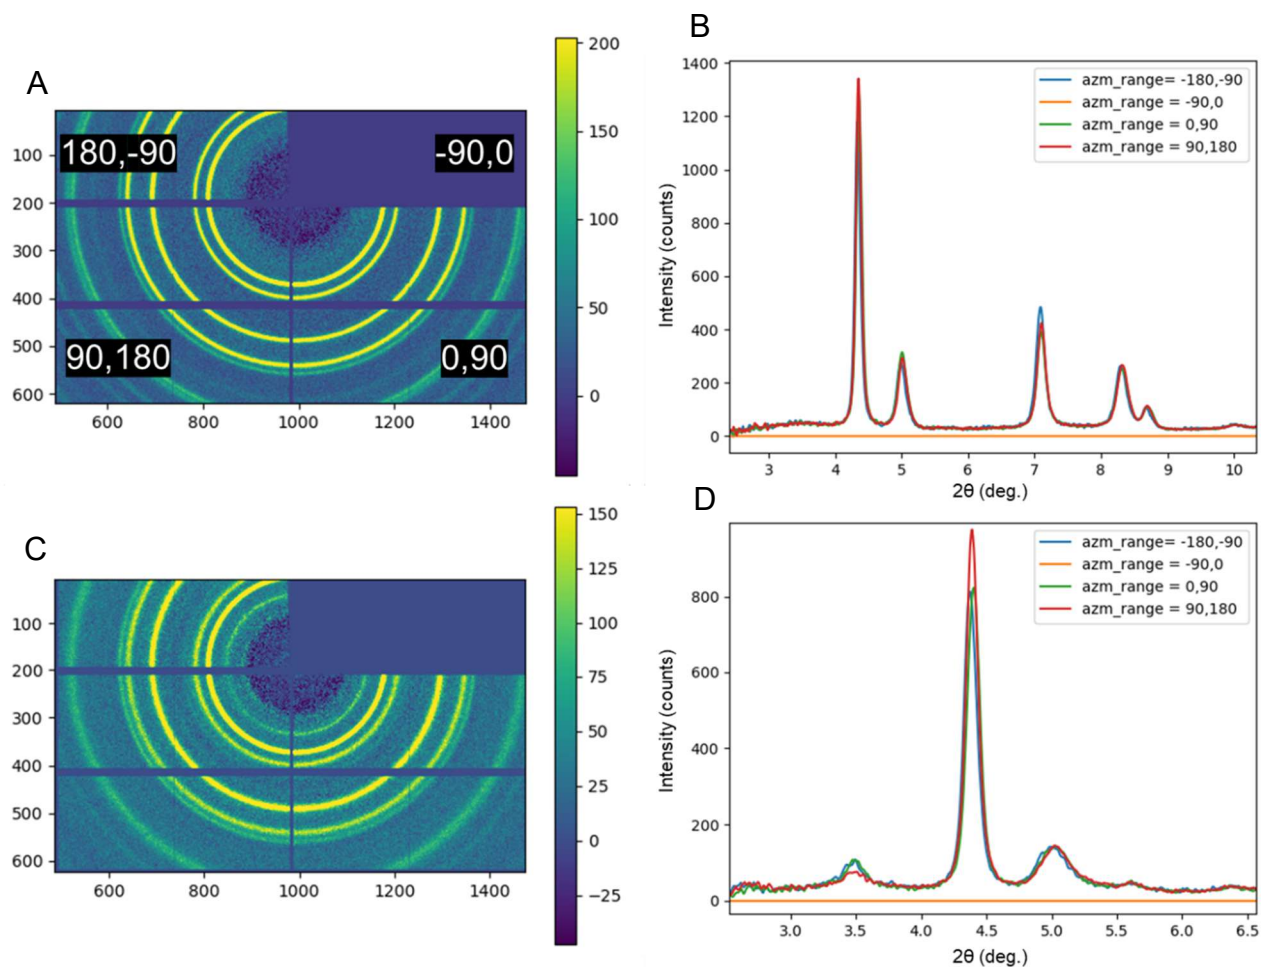

**Figure S10.** Analysis of texture in 2D diffraction images collected on the Al-Ni-Pt combinatorial library ( $\lambda = 0.1665 \text{ \AA}$ ). (A) Example image collected near the Ni deposition site and (B) corresponding integrated patterns from azimuthal slices showing minimal texture. (C) Example image collected near the film center showing texture on low-angle rings and (D) corresponding integrated patterns from azimuthal slices showing texture on multiple peaks.

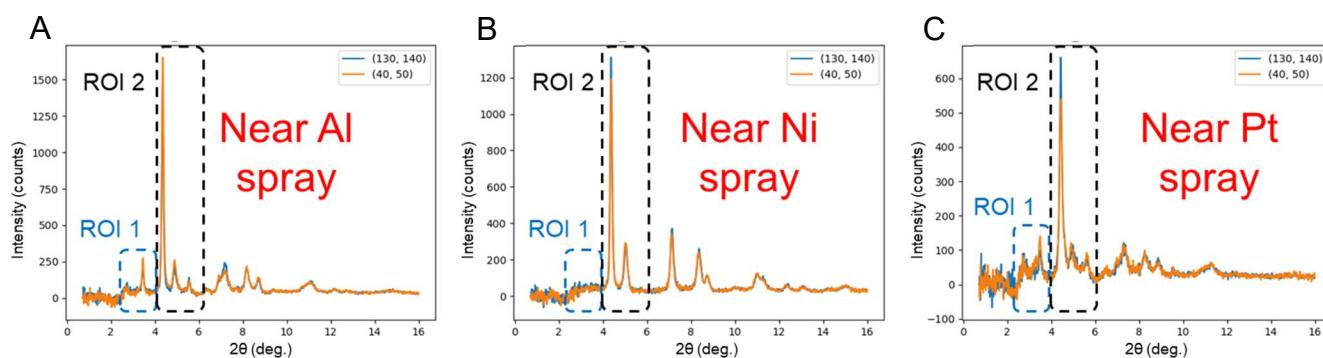

**Figure S11.** Comparison of integrated 1D diffraction patterns ( $\lambda = 0.1665 \text{ \AA}$ ) using azimuthal slices from  $130^\circ - 140^\circ$  (blue) and  $40^\circ - 50^\circ$  (orange). Example patterns shown from data collected near (A) the Al deposition, (B) the Ni deposition, and (C) the Pt deposition. ROI 1 is in the  $2\theta$  range of  $2.5^\circ - 3.9^\circ$  and provides sensitivity to the face-centered tetragonal peaks, while ROI 2 is in the  $2\theta$  range of  $3.9^\circ - 6.1^\circ$  and is sensitive to intensity variations for the most intense face-centered cubic peak which overlaps a face-centered tetragonal peak.

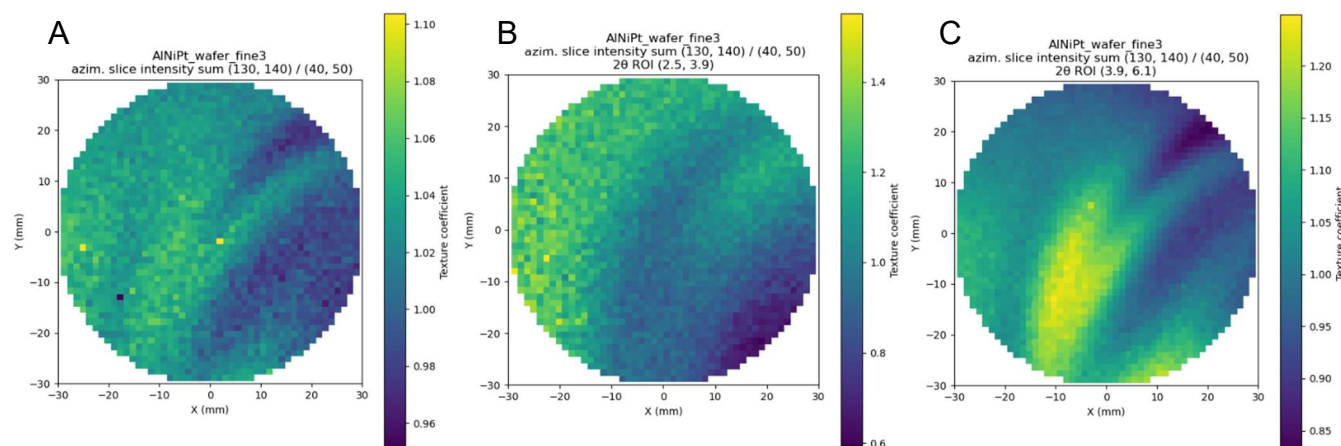

**Figure S12.** Comparison of texture coefficient that approximates the azimuthal intensity variation. Texture coefficient is calculated by dividing the summed intensity in the 1D pattern integrated using an azimuthal range of  $130^\circ - 140^\circ$  by the summed intensity in the 1D pattern integrated using an azimuthal range of  $40^\circ - 50^\circ$ . (A) Texture coefficient from comparing the full  $2\theta$  range of patterns integrated with different azimuthal ranges. (B) Texture coefficient from comparing the summed intensities in ROI 1 ( $2.5^\circ - 3.9^\circ$ ,  $2\theta$ ) for patterns integrated with different azimuthal ranges, providing sensitivity to intensity variations in the low-angle face-centered tetragonal peaks. (C) Texture coefficient from comparing the summed intensity in ROI 2 ( $3.9^\circ - 6.1^\circ$ ,  $2\theta$ ) for patterns integrated with different azimuthal ranges, providing sensitivity to the most intense peak shared by the face-centered cubic and face-centered tetragonal phases.

## Simulation of an Al-Li-Fe oxide combinatorial library and *in silico* AI-driven experiments

While the optimal AI agent(s) for driving valuable measurement campaigns will differ for a given sample, dataset, and experimental technique, we have demonstrated that off-the-shelf machine learning models can be easily plugged into our framework for testing and development. Our fully AI-driven measurement approach used a Gaussian process classifier with a radial basis function kernel, the probabilistic predictions of the classifier, and the Shannon entropy (*i.e.*, uncertainty) associated with those predictions to select measurements. In addition to uncertainty, an edge detection algorithm identified points as on / off an edge by comparing the labels predicted at each point to the labels of neighboring points. This edge characteristic is then normalized and combined with the normalized GPC prediction uncertainty to enhance features in the cumulative distribution function from which measurements are sampled.

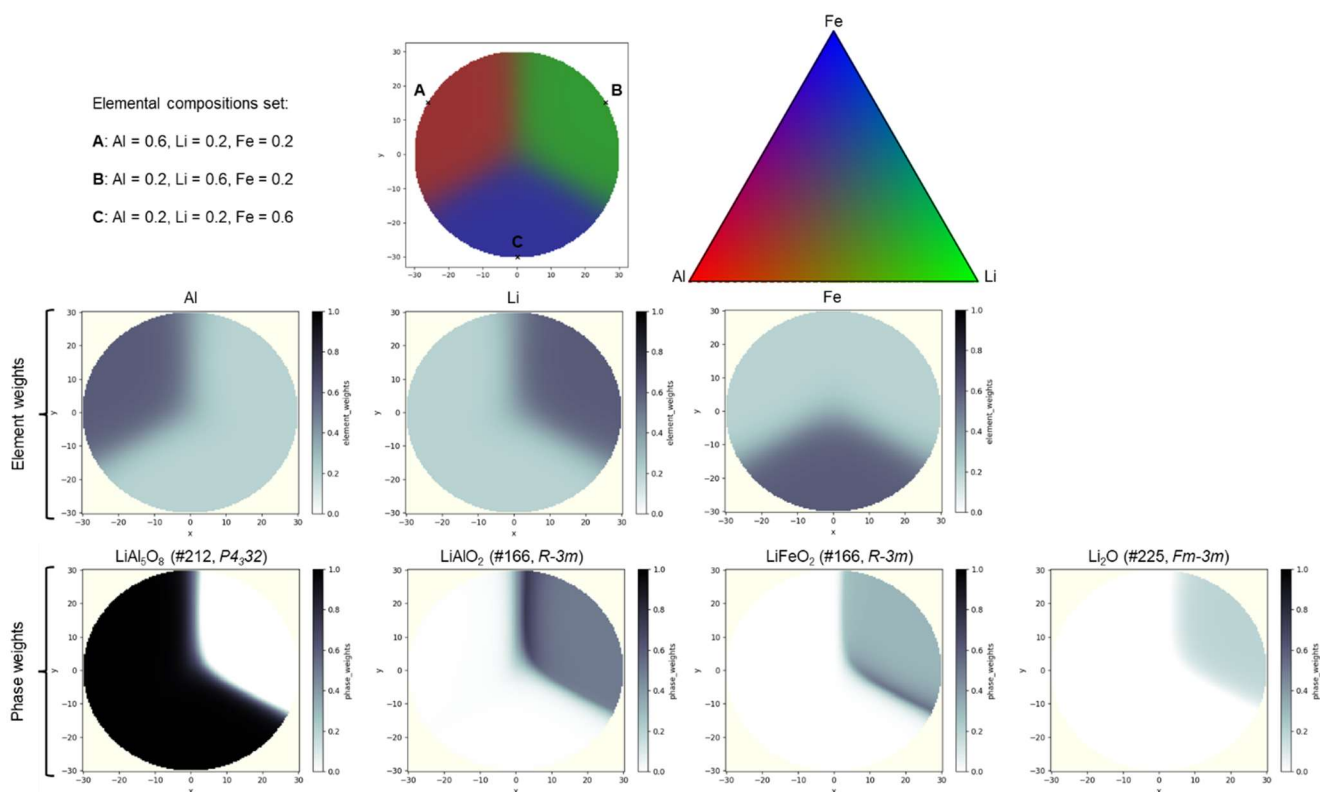

**Figure S13.** Simulated composition spread and phase distributions for a combinatorial library in the ternary Al-Li-Fe oxide system. (Top) Composition set at fixed coordinates A, B, and C on grid and corresponding composition mixtures across wafer indicated on ternary phase diagram colormap. (Middle) Individual element distributions across simulated sample. (Bottom) Individual phase distributions across simulated sample.



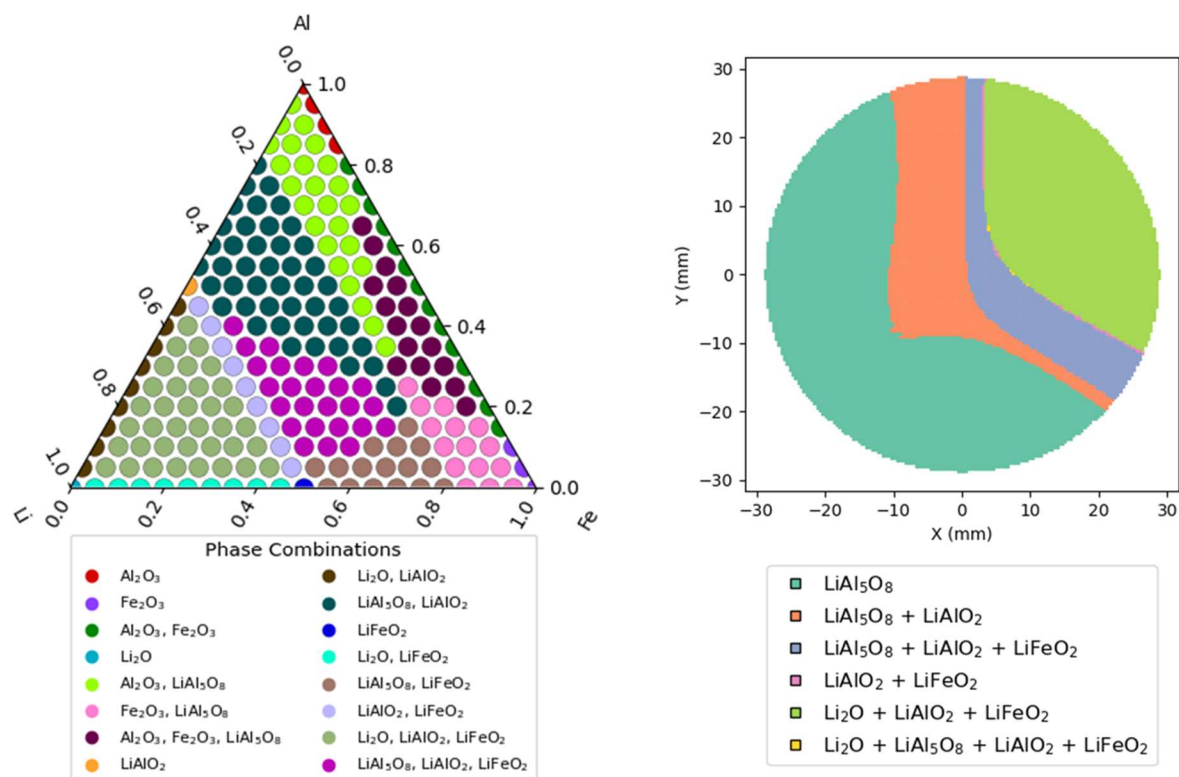

**Figure S14.** (Left) Phases present as a function of composition in the Al-Li-Fe oxide system. (Right) Simulated wafer with points colored by the unique combination of phases.

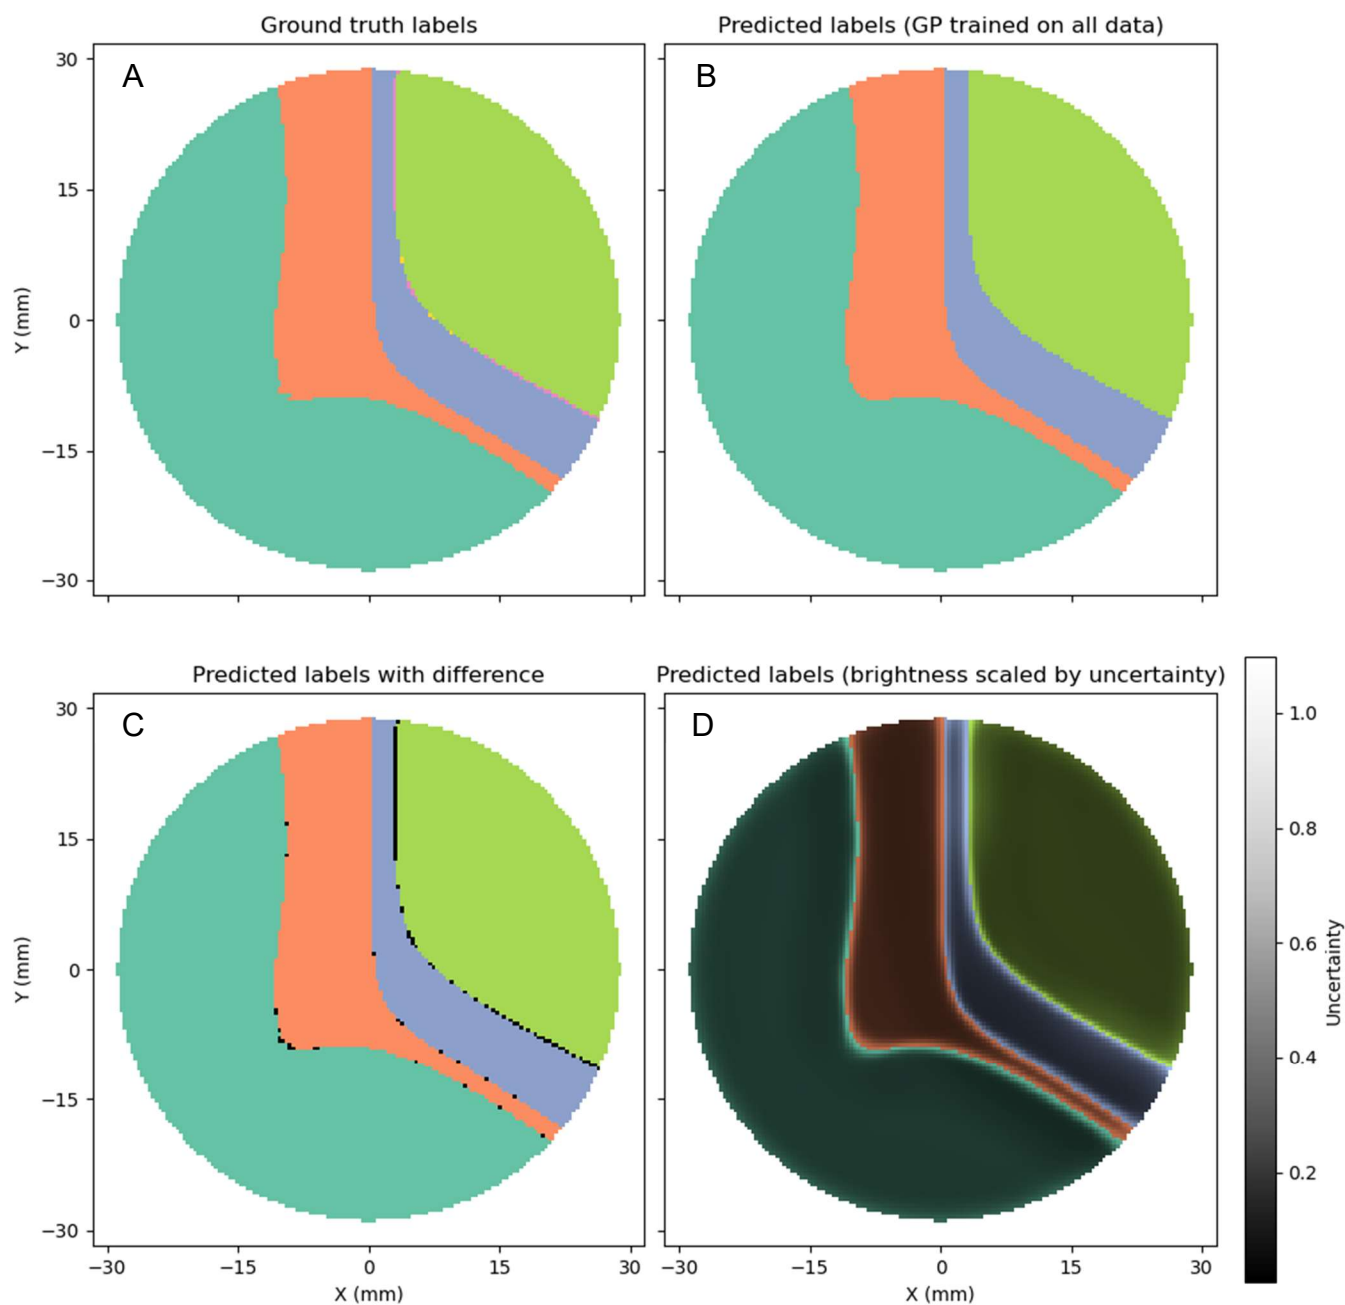

**Figure S15.** Comparison of A) the simulated Al-Li-Fe oxide sample with colors corresponding to the ground truth labels and B) the best possible model predicted by the GP classifier trained on all  $x,y$  coordinates and assigned ground truth labels. C) Model with incorrectly predicted coordinates along borders (black pixels). D) Model with brightness of each point scaled by its uncertainty demonstrating that uncertainty is highest at the borders between regions.

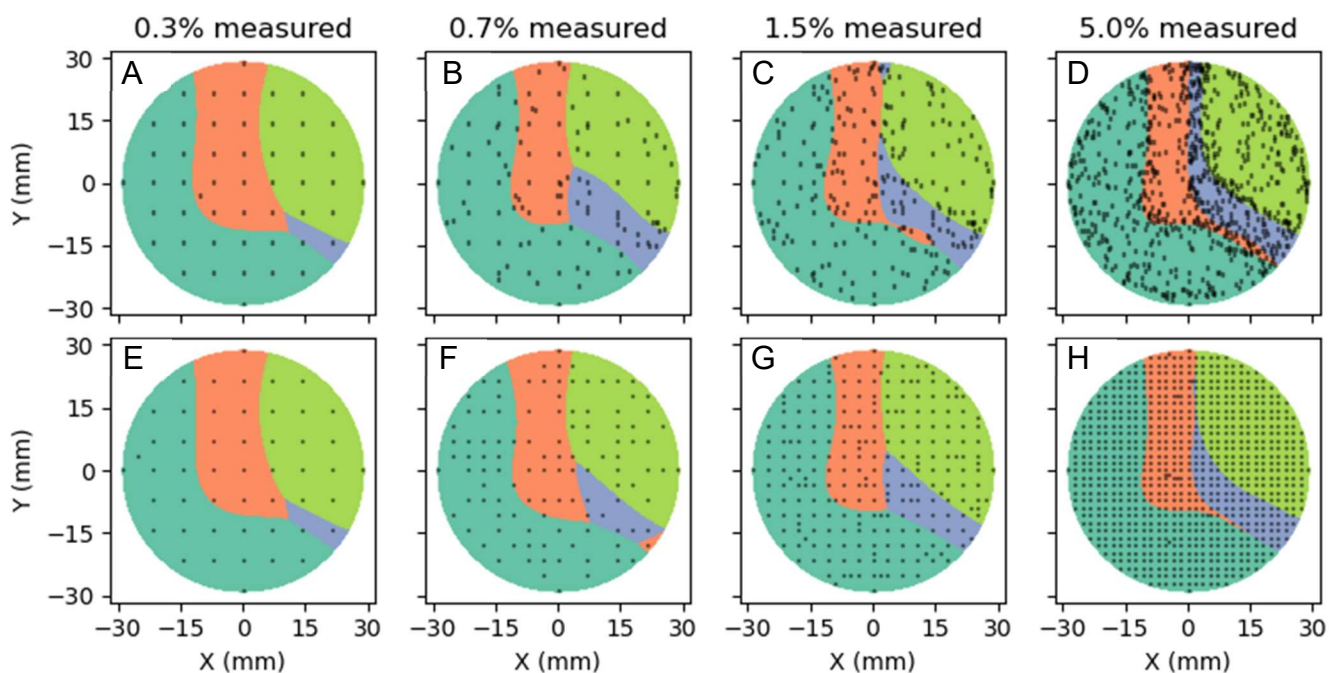

**Figure S16.** Snapshots of simulated experiment campaign progress using (A-D) an AI-driven approach and (E-H) a conventional geometric series. Models of the simulated sample predicted by a Gaussian process classifier trained on measured coordinates and labels after collecting (A, E) 0.3 %, (B, F) 0.7 % (C, G) 1.5 %, and (D, H) 5.0 % of total possible measurements. Measured coordinates shown as pixels outlined in black.

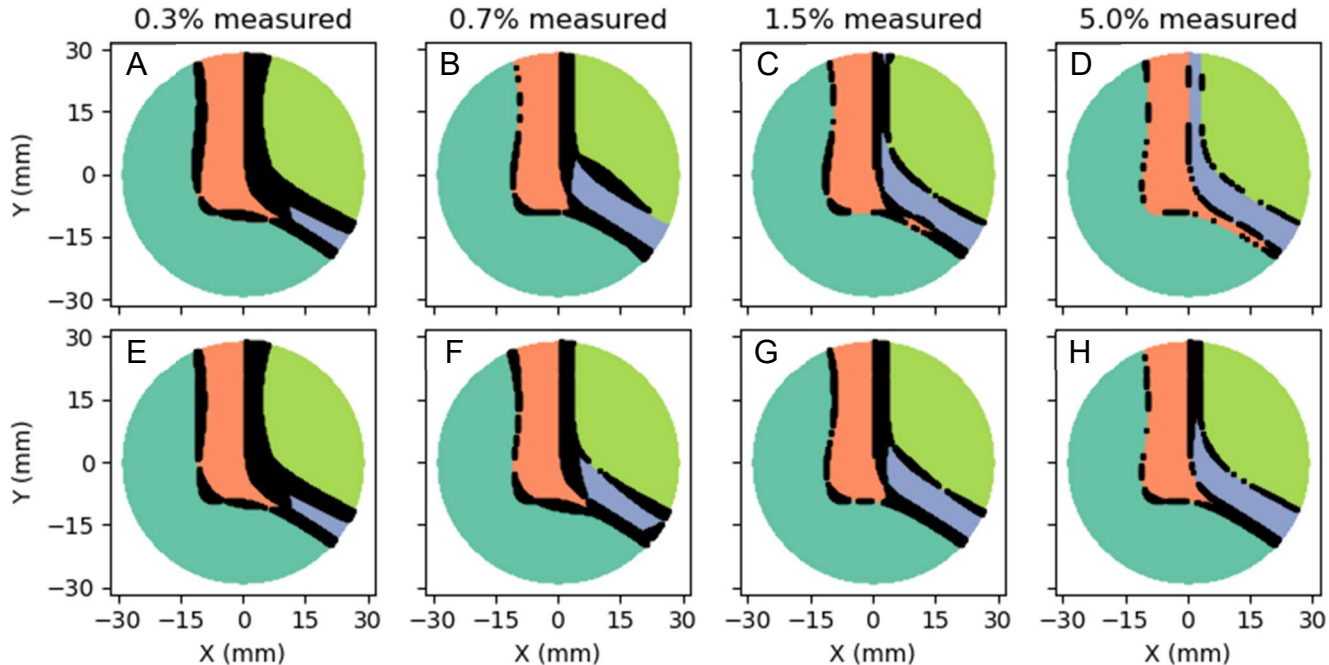

**Figure S17.** Snapshots of simulated experiment campaign progress using (A-D) an AI-driven approach and (E-H) a conventional geometric series. Models of the simulated sample predicted by a Gaussian process classifier trained on measured coordinates and labels after collecting (A, E) 0.3 %, (B, F) 0.7 % (C, G) 1.5 %, and (D, H) 5.0 % of total possible measurements. Mislabeled coordinates shown as black pixels to highlight differences between the ground truth (Figure 8) and models.

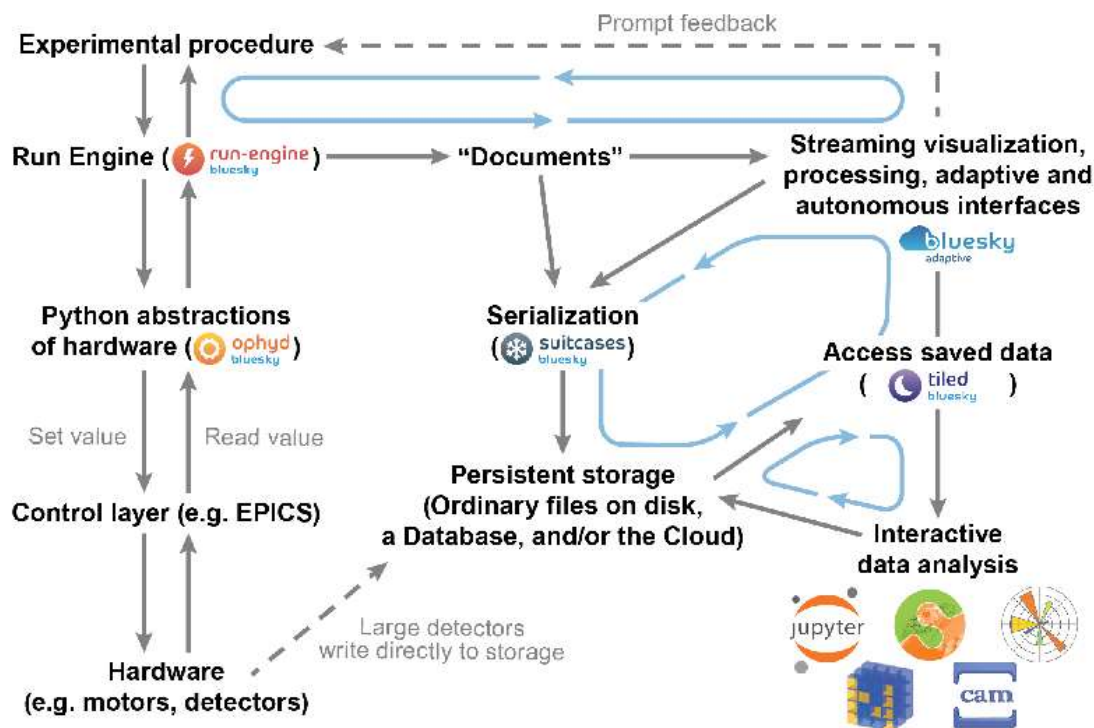

**Figure S18.** Separable pieces of the Bluesky project that may be used, extended, or replaced. Development within the Python ecosystem enables interoperability with existing and future libraries and tools. AI agents are included as part of the top right section for adaptive and autonomous interfaces.

## References

- [1] B. Ravel, M. Newville, *J Synchrotron Radiat* 2005, *12*, 537.
- [2] A. G. McKale, B. W. Veal, A. P. Paulikas, S.-K. Chan, G. S. Knapp, *Phys Rev B* 1988, *38*, 10919.
- [3] S. I. Zabinsky, J. J. Rehr, A. Ankudinov, R. C. Albers, M. J. Eller, *Phys Rev B* 1995, *52*, 2995.
- [4] J. L. Kamm, W. W. Milligan, *Scripta Metallurgica et Materialia* 1994, *31*, 1461.
- [5] S. Hayashi, S. I. Ford, D. J. Young, D. J. Sordellet, M. F. Besser, B. Gleeson, *Acta Mater* 2005, *53*, 3319.
- [6] B. Gleeson, N. Mu, S. Hayashi, *J Mater Sci* 2009, *44*, 1704.
- [7] X. G. Lu, B. Sundman, J. Agren, *CALPHAD* 2009, *33*, 450.
- [8] B. Grushko, D. Kapush, L. Meshi, *J Alloys Compd* 2012, *514*, 60.
- [9] B. Grushko, D. Kapush, *J Alloys Compd* 2014, *594*, 127.
- [10] A. A. Popov, A. D. Varygin, P. E. Plyusnin, M. R. Sharafutdinov, S. V. Korenev, A. N. Serkova, Y. V. Shubin, *J Alloys Compd* 2022, *891*, 161974.
- [11] H. Meininger, M. Ellner, *J Alloys Compd* 2003, *353*, 207.
- [12] G. H. Cao, Z. Zhang, X. Li, W. Skrotzki, E. Müller, R. Schneider, D. Gerthsen, *Acta Mater* 2021, *207*, 116703.
- [13] P. Bordeenithikasem, J. Liu, S. A. Kube, Y. Li, T. Ma, B. E. Scanley, C. C. Broadbridge, J. J. Vlassak, J. P. Singer, J. Schroers, *Sci Rep* 2017, *7*, 7155.
- [14] S. A. Kube, S. Sohn, D. Uhl, A. Datye, A. Mehta, J. Schroers, *Acta Mater* 2019, *166*, 677.
- [15] P. W. Stephens, *J Appl Crystallogr* 1999, *32*, 281.
